# Supplementary material for: Path to perfect photon entanglement with a quantum dot
Source: arXiv:1710.10815 ancillary file (2017-10-30)
Supplement: Supplementary file 1 [file Supplementary.pdf]

# Supplementary Information
## Path to perfect photon entanglement with a quantum dot

A. Fognini[1], A. Ahmadi[2], M. Zeeshan[3], J. T. Fokkens[1], S. J. Gibson[3], N. Sherlekar[3], S. J. Daley[3], D. Dalacu[4], P. J. Poole[4], K. D. Jöns[5], V. Zwiller[1,5], and M. E. Reimer[3]

[1] *Kavli Institute of Nanoscience Delft, Delft University of Technology, Delft 2628 CJ, The Netherlands*
[2] *Institute for Quantum Computing and Department of Physics & Astronomy, University of Waterloo, Waterloo, ON N2L 3G1, Canada*
[3] *Institute for Quantum Computing and Department of Electrical & Computer Engineering, University of Waterloo, Waterloo, ON N2L 3G1, Canada*
[4] *National Research Council of Canada, Ottawa, ON K1A 0R6, Canada*
[5] *Department of Applied Physics, Royal Institute of Technology (KTH), AlbaNova University Center, SE - 106 91 Stockholm, Sweden*

# 1 Power Dependence of Exciton and Biexciton

Fig. 1 (a) depicts the power dependent $g^{(2)}$ of the exciton excited at 870 nm, and Fig. 1 (b) shows the same for the biexciton line. The single photon purity of the exciton lies below 1 %, even above saturation, whereas for the biexciton it saturates at 10 % because of reexcitation. Fig. 1 (c) shows the detected count rates of the X and XX line at 830 nm excitation as a function of excitation power. The numbers indicate the slopes of the curves in the log-log graph, which are close to what is expected (slope of 1 for the exciton and 2 for the biexciton). Fig. 1 (d) shows the detected count rates for X and XX in the case of 870 nm excitation as a function of excitation power. Here, the slopes as well as the saturation behavior differ from Fig. 1 (c). The slopes are smaller and the saturation is less pronounced. In case of non-resonant excitation at the saturation power the single photon purity of the exciton is still below 1 % and the biexciton yields $g^{(2)}_{XX} = 0.1$.

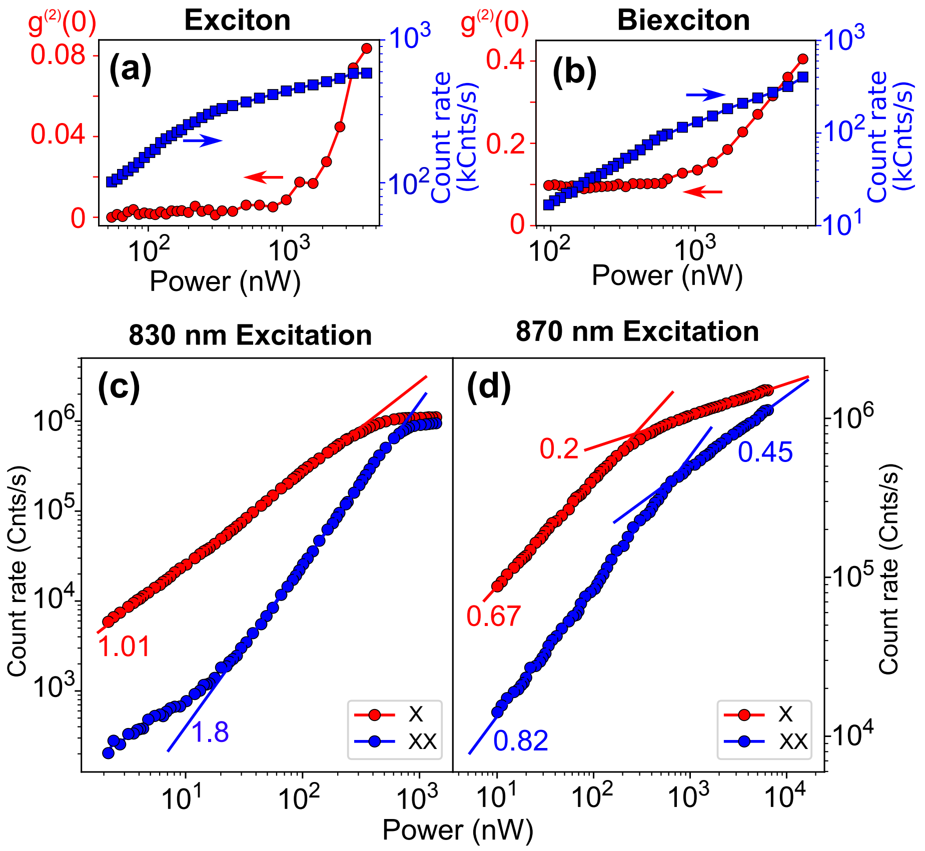


Figure 1: Power dependence of the $g^{(2)}(0)$ excited at quasi resonance (870 nm) for **(a)** the exciton, and **(b)** the biexciton. **(c)** Power dependence dependent count rates of the exciton and the biexciton line at non-resonant excitation (830 nm). **(d)** Power dependent count rates of the exciton and the biexciton line at quasi-resonant excitation (870 nm). The numbers next to the lines indicate the slope on the log-log plot.

## 2 Quantum Dot Characteristics

The QD spectrum changed considerably by tuning from non-resonant excitation (830 nm) to quasi-resonant (870 nm), compare Fig. 1 in the main text.

We wanted to know whether the line at which we excited at 870 nm originated from the QD's p-shell or from donor/acceptor exciton transitions [1] within the InP nanowire. We investigated this question by exciting the QD at low power ($\sim$ 15nW) at 820 nm. If it was a p-shell transition the line should disappear since an exciton in the p-shell would immediately relax to the s-shell. In our case, we still see the line at low power indicative for a donor/acceptor exciton transition [1]. This implies that we did not excite directly at the p-level. This conclusion is further corroborated by cross-correlation measurements where we found that all of the emission lines around 870 nm were uncorrelated with the QD s-shell.

We further investigated the dynamics of the InAsP QD at quasi-resonance by performing cross-correlations between all of the emission lines in the QD s-shell. Fig. 2 shows the result of the cross-correlations between $X, XX, X^-$, and $X^+$. The cascades were fitted using an exponential-Gaussian hybrid [2]. In each cascade the area of the center peak was compared to the average area of the side peaks (uncorrelated coincidence counts) by calculating their ratio. We have defined the area as the part until the curve falls below the full width at half maximum (FWHM) point. In this way, we can circumvent problems when the lifetime overlaps with the adjacent peak (e.g. Fig. 2 (e)). These measurements imply that the holes are trapped at a higher rate than electrons. This finding is in agreement with our sample being unintentionally n-doped whereby the QD's s-level is already filled with electrons without laser excitation.

In summary we find:

1. The lines at 870 nm are not p-shell resonances from the QD, but donor/acceptor exciton transitions [1] within the wurtzite InP nanowire.
2. Both electrons and/or holes get trapped in the QD after a radiative decay.
3. Holes are trapped faster than electrons as indicated by the shorter decay time of 0.81 ns in Fig. 2 (d) as compared to 5.5 ns in Fig. 2 (e).

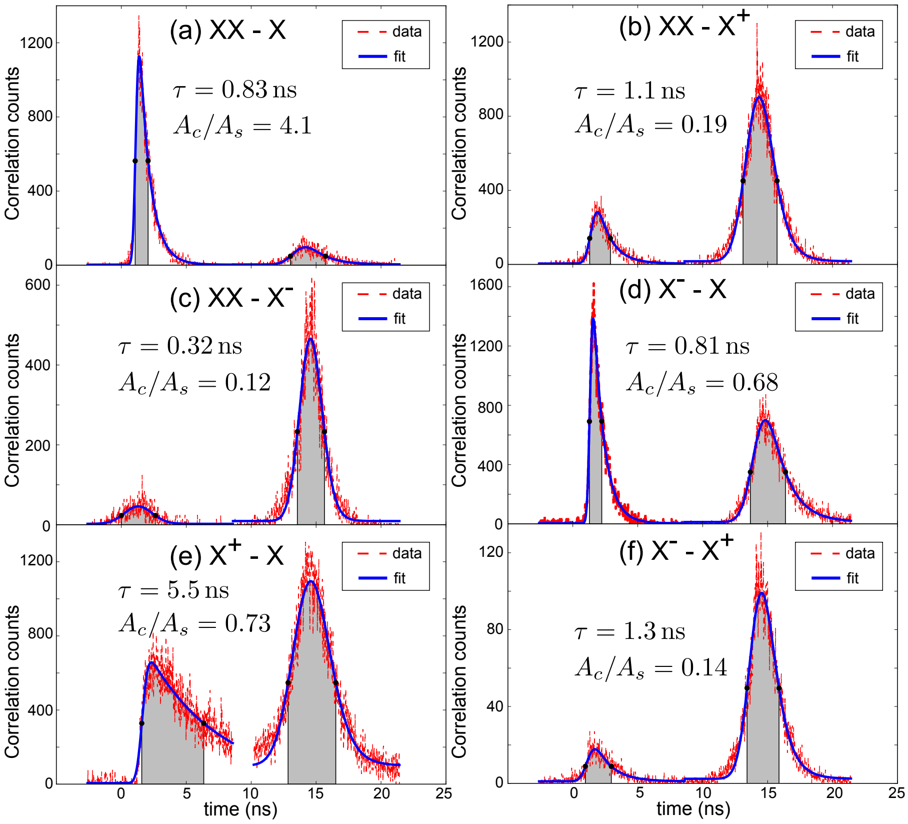


Figure 2: In all figures $\tau$ is the time scale of the decay and $A_c$ is the area in the FWHM region for the central peak, whereas $A_s$ is the area in the FWHM region for the side peak. **(a)** Shows the $XX - X$ cascade as a reference. **(b)** Shows the cascade between $XX$ and $X^+$ (starting on $XX$ and stopping on $X^+$). This shows that after the emission of $XX$, in a time scale of about 1 ns, a hole can get trapped in the QD. **(c)** Depicts the cross-correlation between the $XX$ and $X^-$. It suggests that the trapping of an electron after a $XX$ decay is almost equally likely as a hole, compare (b). **(d)** Shows cross-correlations between $X^-$ and $X$. **(e)** Shows the correlations between $X^+$ and $X$. Comparing this graph with (d) indicates that the rate at which electrons get trapped is slower than holes (0.83 ns compared to 5.5 ns). **(f)** Shows the $X^-$ to $X^+$ cross-correlations. The numbers indicate that the process of trapping two holes within the laser repetition rate is suppressed. In all panels the first state is the start photon and the second state is the stop photon for the cross-correlation measurements.

# 3 Tomography Setup Calibration

The quantum state tomography setup was built according to Ref. [3], compare Fig. 3. A crucial part before performing the correlation measurements is the calibration of the waveplates and polarizers. Any miscalibration reduces the quality of the quantum state tomography.

The calibration was performed in three steps:

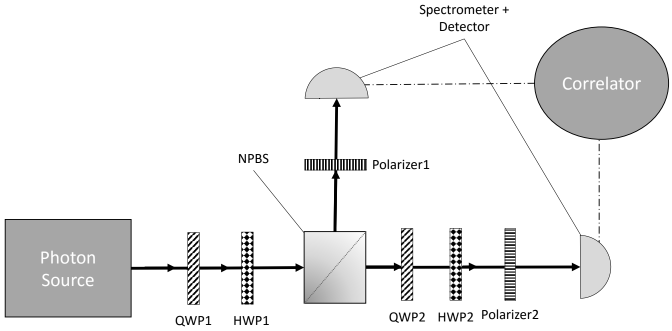


Figure 3: Schematic view off the setup used to analyzed the entangled photon pairs following Ref. [3]. The setup includes a pair of polarizers, a pair of half-waveplates (HWPs), a pair of quarter-waveplates (QWPs), a non-polarizing beam splitter (NPBS), a pair of spectrometers, single photon detectors, and finally a correlator to build the histogram from the signals of the detectors. The two polarizers are set to $H$ polarization.

1. **Polarization reference:** A polarizing beamsplitter served as the vertical polarization (V) reference. It was directly placed on the optical table and aligned carefully along the incoming laser beam (870 nm). In this case it only transmitted V-polarized light and we used it as the polarization reference for the polarizer calibration.

2. **Polarizer calibration:** The polarizers were calibrated to H-polarization (defined to be parallel to the optical table). The polarizers were adjusted until the V-polarized light transmission was minimal.

3. **Waveplate calibration:** Each of the two $\lambda/2$ and $\lambda/4$-waveplates were calibrated individually to find their zero-point. They were placed between the polarizing beamsplitter and the aligned polarizer. They were rotated till minimal light transmission through the polarizer was achieved which is their zero-point.

To test the waveplate's and polarizer's calibration we performed a quantum state tomography [4] in all 36 bases (HH, HV, ...) on classical H-polarized laser light (870 nm). The measurement result is depicted in Fig. 4 and shows only a clean peak at $|HH\rangle\langle HH|$ highlighting a very good calibration of our state analysis system. The fidelity between the measured density matrix and the density matrix describing purely $H$ polarized light is 0.993. This very high number (in the ideal case one) reveals a very well aligned setup.

The waveplate settings to perform the 36 bases quantum tomography are listed in Table 3. They were calculated based on Ref. [5].

| **Basis** | $\mathbf{QP}_1$ | $\mathbf{HP}_1$ | $\mathbf{QP}_2$ | $\mathbf{HP}_2$ | **Basis** | $\mathbf{QP}_1$ | $\mathbf{HP}_1$ | $\mathbf{QP}_2$ | $\mathbf{HP}_2$ |
|---|---|---|---|---|---|---|---|---|---|
| HH | 0 | 0 | 0 | 0 | HV | 0 | 0 | 0 | 45 |
| HD | 0 | 0 | −45 | 0 | HA | 0 | 0 | 0 | −22.5 |
| HR | 0 | 0 | −45 | −22.5 | HL | 0 | 0 | −45 | 22.5 |
| VH | 0 | 45 | 0 | 45 | VV | 0 | 45 | 0 | 0 |
| VD | 0 | 45 | −45 | 0 | VA | 0 | 45 | 0 | −22.5 |
| VR | 0 | 45 | −45 | 22.5 | VL | 0 | 45 | −45 | −22.5 |
| DH | −45 | 22.5 | −45 | 0 | DV | −45 | 22.5 | 0 | −22.5 |
| DD | −45 | 22.5 | 0 | 0 | DA | −45 | 22.5 | 0 | 45 |
| DR | −45 | 22.5 | −45 | 22.5 | DL | −45 | 22.5 | −45 | −22.5 |
| AH | −45 | −22.5 | −45 | 0 | AV | −45 | −22.5 | 0 | −22.5 |
| AD | −45 | −22.5 | 0 | 45 | AA | −45 | −22.5 | 0 | 0 |
| AR | −45 | −22.5 | −45 | −22.5 | AL | −45 | −22.5 | −45 | 22.5 |
| RH | −45 | 0 | −45 | 0 | RV | −45 | 0 | 0 | −22.5 |
| RD | −45 | 0 | −45 | −22.5 | RA | −45 | 0 | −45 | 22.5 |
| RR | −45 | 0 | 0 | 0 | RL | −45 | 0 | 0 | 45 |
| LH | 0 | −22.5 | −45 | −22.5 | LV | 0 | −22.5 | −45 | 22.5 |
| LD | 0 | −22.5 | −45 | 0 | LA | 0 | −22.5 | 0 | −22.5 |
| LR | 0 | −22.5 | 0 | 45 | LL | 0 | −22.5 | 0 | 0 |

Table 1: Summarizing all waveplate angle settings in degrees used to perform the full set of correlation measurements. Here, QP and HP are the abbreviations for $\lambda/4$- and $\lambda/2$-waveplates, respectively. The subscript numbers match the numbers in the setup schematic, compare Fig. 3.

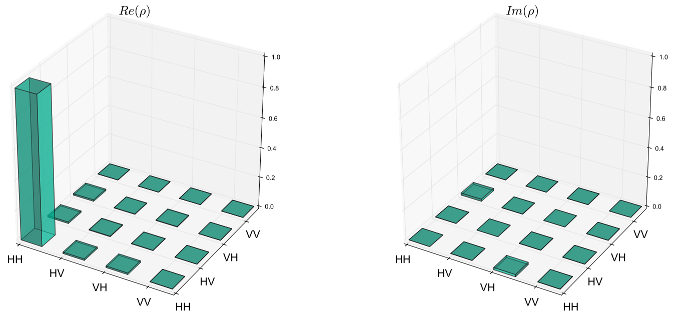


Figure 4: Tomography of $H$ polarized laser pulses. The fidelity between the measured density matrix and a density matrix describing purely $H$ polarized light is 0.993. Since the imaginary part of the density matrix is negligible, $\leq 1\%$, no phase is introduced by the NPBS, QWPs, HWPs, and the polarizers.

# 4 Correlation Measurements

Fig. 5, 6, and 7 depict the raw data of all 36 correlation measurements used for the quantum state tomography shown in Fig. 2, 4 (a), and 4 (b) in the main text, respectively. The data was recorded with 16 ps time bins.

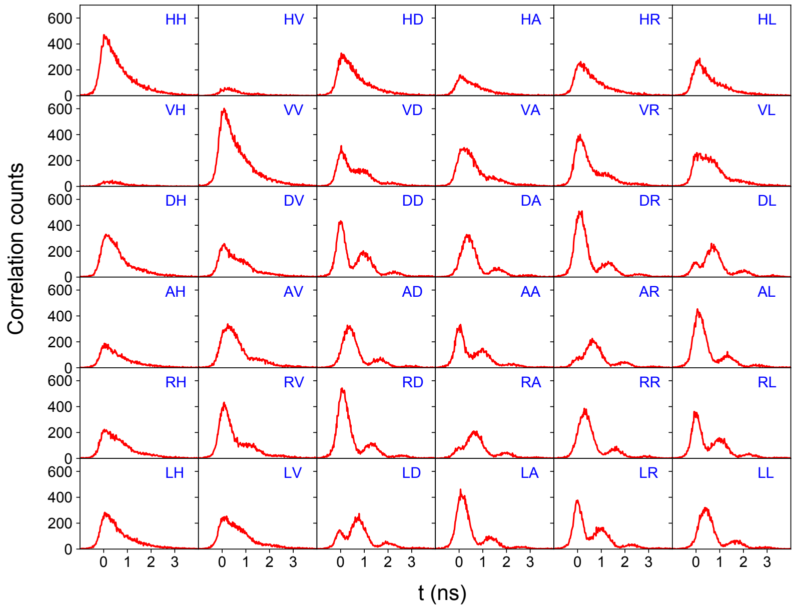


Figure 5: Quasi-resonant excitation at 870 nm was employed. The figure depicts the raw data used for the quantum state tomography measurements presented in Fig. 2 of the main text. The integration time per basis was 370 s.

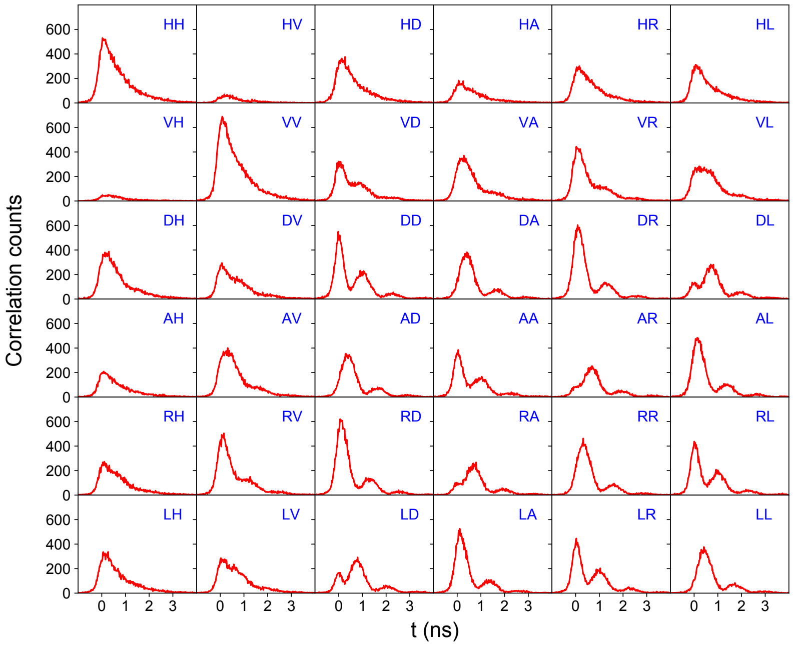


Figure 6: Quasi-resonant excitation at 870 nm was employed. The figure depicts the raw data used for the quantum state tomography measurements presented in Fig. 4 (a) of the main text. The integration time per basis was 342 s.

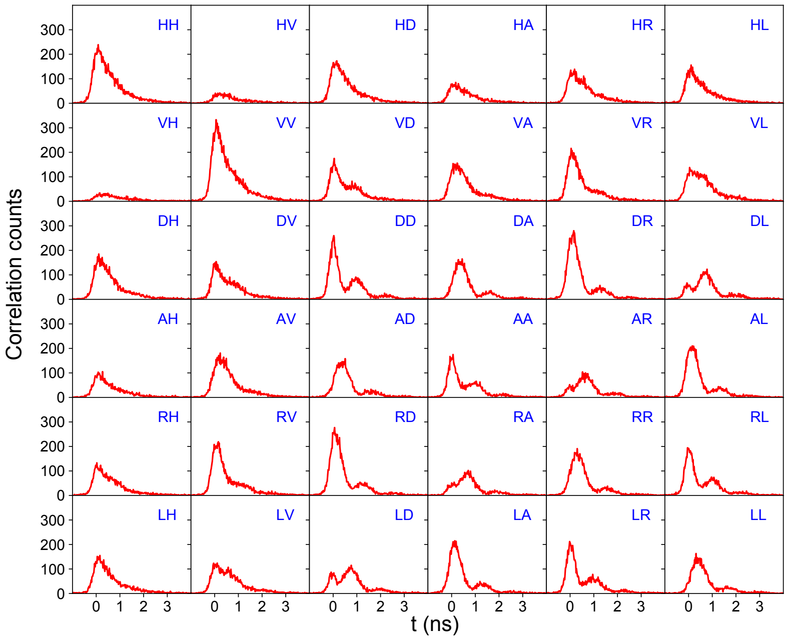


Figure 7: Non-resonant excitation at 830 nm. The figure depicts the raw data used for the quantum state tomography measurements presented in Fig. 4 (b) of the main text. The integration time per basis was 342 s.

# 5 Birefringence

Previous studies on InAsP/InP nanowire quantum dots [3, 6] have shown the effect of birefringence in the nanowire on the quantum state. We investigated if this is also the case in our nanowire. We applied a magnetic field of 4 T along the nanowire's growth direction and analyzed the polarization state of the split exciton ($X$) and biexciton line ($XX$).

In case of no birefringence, we expect the Zeeman-split lines to be fully circularly polarized because of angular momentum conservation. Fig. 8 depicts the photoluminescence (PL) recorded at 830 nm excitation and an applied magnetic field of 4 T. The red line shows the PL when the polarization analyzer only passed right polarized (R) photons and the dashed blue line if the analyzer only passed left polarized (L) photons. We observe that the Zeeman-split lines are either R- or L-polarized, compare Tab. 5 for the extinction ratio values. This shows that our investigated nanowire induces an insignificant amount of birefringence.

This implies that we expect to measure a quantum state of the form

$$|\Psi\rangle = \frac{1}{\sqrt{2}} \left(|RL\rangle + |LR\rangle\right) = \frac{1}{\sqrt{2}} \left(|HH\rangle + |VV\rangle\right), \tag{1}$$

in the case of no fine-structure splitting.

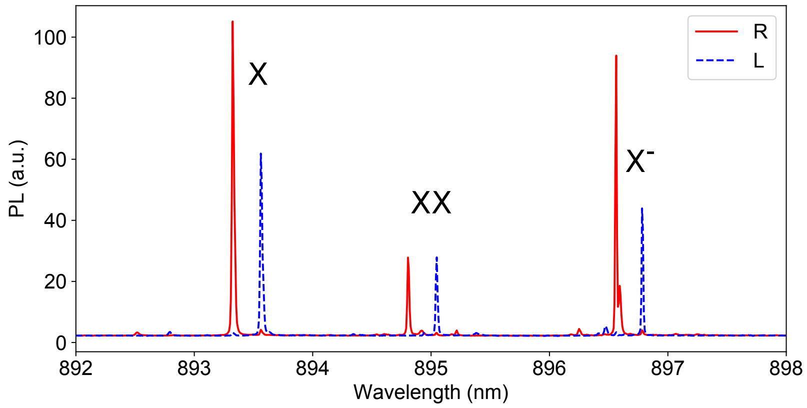


Figure 8: Excitation at 830 nm with an applied magnetic field of 4 T along the nanowire's growth direction. The exciton ($X$), the biexciton ($XX$), and the trion ($X^-$) split in two lines.

| Peak | Extinction ratio in % |
|---|---|
| X Left | $1.03 \pm 0.03$ |
| X Right | $3.32 \pm 0.08$ |
| XX Left | $0.85 \pm 0.06$ |
| XX Right | $3.76 \pm 0.12$ |

Table 2: Polarization extinctions for the exciton (X) and biexciton (XX) lines shown in Fig. 8. The extinction ratio is defined here as the power of the suppressed peak divided by the power of the cross-polarized peak.

# 6 Detector Time Resolution Function

The simulation crucially depends on the used detection system's time resolution function $g(t)$. It cannot be measured with picosecond laser pulses as these pulses are spectrally too different from the QD's emission profile. The reason is that chirp introduced at the spectrometer's gratings changes the pulse length too much in case of short laser pulses.

The only valid way to extract the detection time resolution function is directly from the set of correlation measurements. Namely, the rising part of the correlations without oscillations, e.g., the $HH$ and $VV$ correlations, allow the extraction of the system's time resolution function $g(t)$. The $HH$ and $VV$ correlation counts are of the form

$$f(t) = \Theta(t)e^{-t/\tau_X} * g(t), \tag{2}$$

where, $\Theta(t)$ is the Heaviside function, $\tau_X$ the exciton lifetime, and $*$ denotes the convolution operator. To simplify the deconvolution process we can approximate equation 2 around time zero as

$$f(t) \approx \Theta(t) * g(t). \tag{3}$$

This approach is valid when the half width at half maximum of $g(t)$ ($\sim 100\,\mathrm{ps}$) is smaller than $\tau_X$ ($847\,\mathrm{ps}$). This is fulfilled in our case. The differentiation of $f(t)$ in equation 3 will then directly yield $g(t)$.

Numerically we performed the following algorithm: The sum of $HH$ and $VV$ correlation yields a better signal to noise ratio than only $HH$ or $VV$ alone. Therefore, we use

$$\tilde{f}(t) = HH + VV. \tag{4}$$

Since $\tilde{f}(t)$ is subjected to noise we use use a Savitzki-Golay filter to smoothen $\tilde{f}(t)$ and yield $f(t)$. This procedure is depicted in Fig. 9 (a). As a next step we perform a numerical stepwise differentiation of $f(t)$ and yield the data in Fig. 9 (b). From $df(t)/dt$ we consider the part from negative times until the maximum, which we call $\tilde{g}(t)$. This function contains the full information of the detection time resolution function $g(t)$. In our case $g(t)$ is a symmetric function since both APDs show the same impulse response. Therefore, we can reconstruct the raw $g(t)$ by mirroring $\tilde{g}(t)$ along its maximum, see Fig. 9 (c). Since the raw $g(t)$ is subjected to noise we fit it with

$$g_f(t, t_0, a) = \frac{a}{\sinh{(t - t_0)}^2} \tag{5}$$

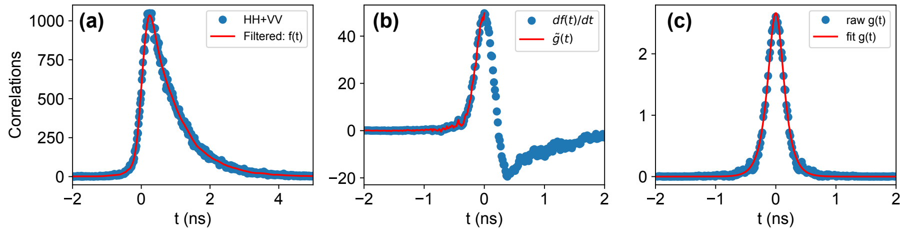


Figure 9: Procedure to acquire the detection system's time resolution function $g(t)$ in order to perform the simulate the concurrence evolution shown in Fig. 2 of the main text. **(a)** The sum of the $HH$ and $VV$ correlations (dots) are smoothed with a Savitzki-Golay filter (red curve) with a polynomial of degree 6 and a window length of 65. **(b)** The filtered correlation data is numerically differentiated (dots) and the part till the maximum (red curve) is the rising part of $g(t)$. **(c)** The dots represent the mirrored $\tilde{g}(t)$. $\tilde{g}(t)$ is fitted with a $\sinh t^{-2}$ function depicted with the red line. A perfect fit is achieved with an $R^2$-value of 0.998.

where $a$ is the amplitude, and $t_0$ the time origin. The fit to the data is in excellent agreement, compare Fig. 9 (c). By normalizing $g_f$ we yield the detection system's time resolution function as

$$g(t) = \frac{g_f(t)}{\int_{-\infty}^{\infty} g_f(t)dt}. \tag{6}$$

Based on $g(t)$ the simulation is performed as described in the main text. This procedure has been applied for all the simulation in the text with a Savitzki-Golay filter with a polynomial of degree 6 and a window length of 65. For the data presented in Fig. 2 of the main text the fit's $R^2$-value is 0.998.

# 7 Count Averaged Concurrence

The count averaged concurrence $\bar{\mathcal{C}}$ in the text is defined as:

$$\bar{\mathcal{C}} := \frac{\sum_{t_k} N^{t_k}\mathcal{C}\left(\rho\left(ij^{t_k}\right)\right)}{\sum_{t_k} N^{t_k}}, \tag{7}$$

where $\rho(ij^{t_k})$ is the density matrix based on the correlation counts $ij^{t_k}$ within a time bin at time $t_k$ $(i,j \in \{H,V,D,A,R,L\})$, $\mathcal{C}$ denotes the concurrence [7], and $N_{t_k}$ is the total correlation counts within a time bin at time index $t_k$, $N^{t_k} = \sum_{i,j} ij^{t_k}$.

# References

[1] B. J. Skromme, T. S. Low, T. J. Roth, G. E. Stillman, J. K. Kennedy, and J. K. Abrokwah, J. Electron. Mater. **12**, 433 (1983).

[2] K. Lan and J. W. Jorgenson, Journal of Chromatography A **915**, 1 (2001).

[3] K. D. Jöns, L. Schweickert, M. A. M. Versteegh, D. Dalacu, P. J. Poole, A. Gulinatti, A. Giudice, V. Zwiller, and M. E. Reimer, Sci. Rep. **7**, 1700 (2017).

[4] T. Fokkens, A. Fognini, and V. Zwiller, (2016-2017), Tomography Library, available at GitHub.

[5] T. Fokkens, A. Fognini, and V. Zwiller, (2016), Waveplates Library, available at GitHub.

[6] M. A. M. Versteegh, M. E. Reimer, K. D. Jöns, D. Dalacu, P. J. Poole, A. Gulinatti, A. Giudice, and V. Zwiller, Nat. Commun. **5**, 5298 (2014).

[7] W. K. Wootters, Phys. Rev. Lett. **80**, 2245 (1998).
